# Supplementary material for: Good Initializations of Variational Bayes for Deep Models
Source: arXiv:1810.08083 source file (2019-01-25)
Supplement: Supplementary file 1 [file all-runs.tex]

\begin{figure*}[t!]
    \centering
    \subfigure{
        \setlength\figureheight{.2\textwidth}
        \setlength\figurewidth{.24\textwidth} 
        \tiny
        \input{../fig/regr-exp/test_5folds_powerplant}
    }
    \subfigure{
        \setlength\figureheight{.2\textwidth}
        \setlength\figurewidth{.24\textwidth} 
        \tiny
        \input{../fig/regr-exp/test_5folds_protein}
    }
    \subfigure{
        \setlength\figureheight{.2\textwidth}
        \setlength\figurewidth{.24\textwidth} 
        \tiny
        \input{../fig/regr-exp/test_5folds_concrete}
    }
    \subfigure{
        \setlength\figureheight{.2\textwidth}
        \setlength\figurewidth{.24\textwidth} 
        \tiny
        \input{../fig/regr-exp/test_5folds_boston}
    }
    \\[-1ex]
    \subfigure{
        \tiny
        \input{../fig/regr-exp/legend}
    }
    \caption{Progression of \rmse and \mnll over training iterations for different initialization strategies on four regression datasets. The neural network architecture used for these experiments has two hidden layers with 50 and 10 hidden neurons and \relu activation functions. The posterior approximation $q_{\theta}(\omegavect)$ of the true distribution $p(\omegavect|\D)$ has fully factorized covariance. Results shown are averaged over 5 different splits of train/test on the entire dataset.}
\end{figure*}

\begin{figure*}[t!]
    \centering
    \subfigure{
        \setlength\figureheight{.2\textwidth}
        \setlength\figurewidth{.25\textwidth} 
        \tiny
        \input{../fig/batchsize-exp/test_5folds_powerplant.tex}
    }
    \subfigure{
        \setlength\figureheight{.2\textwidth}
        \setlength\figurewidth{.25\textwidth} 
        \tiny
        \input{../fig/batchsize-exp/test_5folds_protein.tex}
    }
    \\[-1ex]
    \subfigure{
        \tiny
        \input{../fig/batchsize-exp/legend}
    }
    \caption{Progression of \rmse and \mnll over training iterations for initialization strategies. The posterior approximation $q_{\theta}(\omegavect)$ of the true distribution $p(\omegavect|\D)$ has fully factorized covariance. Results shown are averaged over 5 different splits of train/test on the entire dataset.  \noteSR{TODO: show the same thing also for MNIST and EEG} }

\end{figure*}

%\clearpage

\begin{figure*}[t!]
    \centering
    \subfigure{
        \setlength\figureheight{.2\textwidth}
        \setlength\figurewidth{.25\textwidth} 
        \tiny
        \input{../fig/depth-exp/test_5folds_powerplant}
    }
    \subfigure{
        \setlength\figureheight{.2\textwidth}
        \setlength\figurewidth{.25\textwidth} 
        \tiny
        \input{../fig/depth-exp/test_5folds_protein}
    }
    \subfigure{
        \setlength\figureheight{.2\textwidth}
        \setlength\figurewidth{.25\textwidth} 
        \tiny
        \input{../fig/depth-exp/test_5folds_spam}
    }
    \subfigure{
        \setlength\figureheight{.2\textwidth}
        \setlength\figurewidth{.25\textwidth} 
        \tiny
        \input{../fig/depth-exp/test_5folds_mnist}
    }
    \\[-1ex]
    \subfigure{
        \tiny
        \input{../fig/depth-exp/legend}
    }
    \caption{Progression of \rmse and \mnll over training iterations for different batch sizes for the initialization with Bayesian Liner Models. The neural network architecture used for these experiments has 10 hidden layers with  10 hidden neurons and \relu activation functions each. The posterior approximation $q_{\theta}(\omegavect)$ of the true distribution $p(\omegavect|\D)$ has fully factorized covariance. Results shown are averaged over 5 different splits of train/test on the entire dataset.}

\end{figure*}
